# Supplementary material for: Deformation-induced topological transitions in mechanical metamaterials and their application to tunable non-linear stiffening
Source: arXiv:2111.05284 ancillary file (2022-04-05)
Supplement: Supplementary file 1 [file SI_Top_Mat_1.pdf]

# Supplementary Information: Deformation-induced Topological Transitions in Mechanical Metamaterials and their Application to Tunable Non-linear Stiffening

Marius Wagner[1*§], Fabian Schwarz[1*§], Nick Huber[1], Lena Geistlich[1], Henning Galinski[1] and Ralph Spolenak[1]

[1]Laboratory for Nanometallurgy, Department of Materials, ETH Zürich
[*]Corresponding authors. E-mails: marius.wagner@mat.ethz.ch; fabian.schwarz@mat.ethz.ch
[§]These authors contributed equally to this work.

## 1 Unit cells undergoing topological transitions

For the design of beam-based metamaterials undergoing transformations in nodal-topology when deformed, it is helpful to think of them as trusses consisting of struts connected by perfect hinges i.e. frictionless pin-joints. When such frameworks are kinematically indeterminate, they contain internal mechanisms; soft, zero-energy modes, which will deform by rotation in the joints while the struts remain unstrained. These inextensional deformation modes allow the movement of joints along a defined trajectory for a given applied load. This can be harnessed to generate transitions in nodal topology, i.e. changes in the connectivity of the framework. By rational design of the unit cell, the trajectories of displacing joints can be controlled such that internal self-contacts are generated. The presented metamaterials are designed, such that the newly formed contacts mutually constrain further displacement of their contact partner. As a result, the soft mode in the framework is frustrated and loads can be transmitted across the contact. Further deformation requires changes in the beam length (rigid, stretch-dominated deformation) instead of rotations in joints (soft, bending dominated deformation). The two joints in contact essentially behave like one single joint, for the given loading scenario.
Unit cells in which internal contact leads to topology transitions are depicted in Figure S1. The design is based on honeycomb structures, containing internal mechanisms.

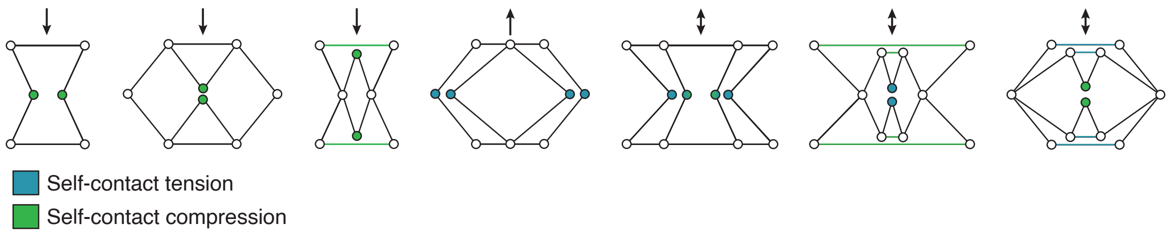


Figure S1: Unit cells based on honeycomb structures undergoing changes in topology when deformed in tension, compression, or both tension and compression.

# 2 Matrix analysis of the topology changing metamaterials

The matrix analysis performed in this study is based on the algorithm of Pellegrino *et al.*[1]. This is used to calculate the inextensional, soft modes of deformation in tension / compression unit cell. The analysis is performed separately for each of the topological states (initial unreformed, tension and compression state). We assume the an idealized metamaeterial consisting of rigid beams connected by frictionless pin joints. The $\psi = 12$ joints in the unit cell are labeled *A* - *L* and the the $\iota = 14$ beams are labeled *a* - *n*, further $\kappa = 5$ kinematic constrains are applied to the joints according to Figure S2. In the following the equilibrium matrices $A$ will be analysed for

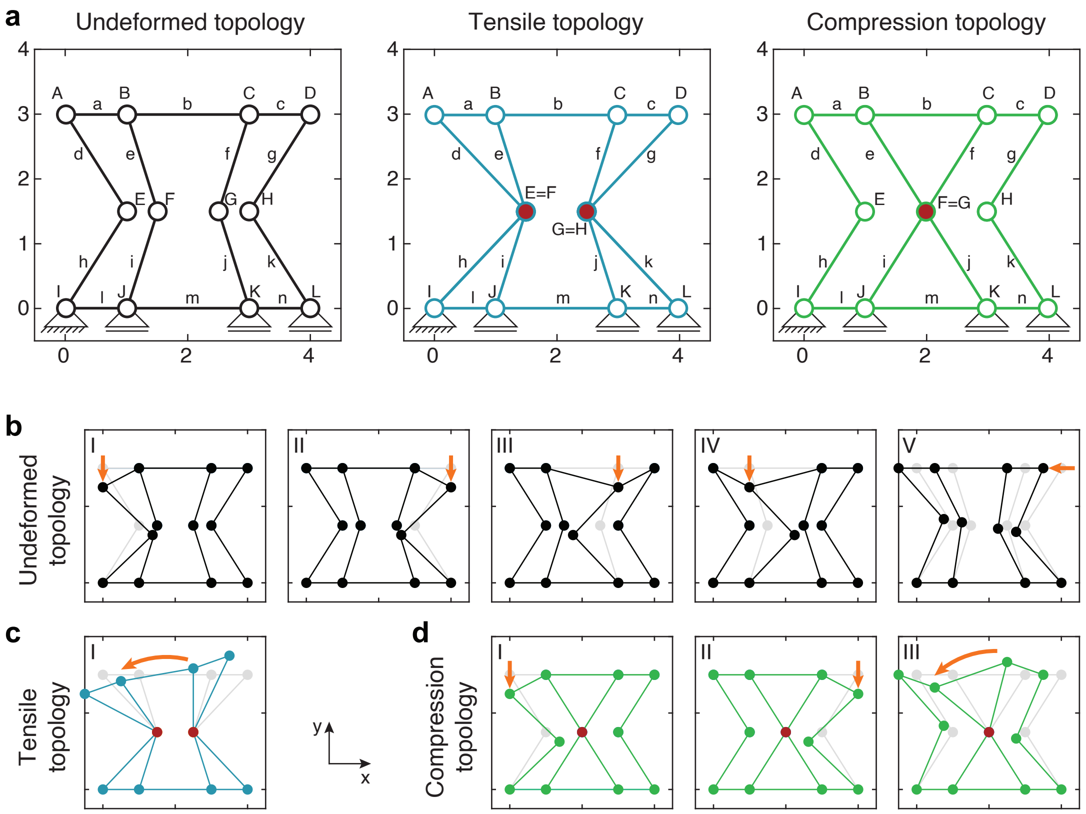


Figure S2: Matrix analysis of tension / compression metamaterial. a) Rigid beam, pin joint representations of the three topological states. Inextensional deformation modes of the initial topology (b), tensile topology (c), and compression topology (d).

the different topologies (initial, tension, and compression). The equilibrium matrix relates the $\iota$ tensions in the beams, assembled in vector $t$, to the $2\psi - \kappa$ components of external forces acting on the joints of vector $f$.

$$A\,t = f \tag{1}$$

The zero-modes, i.e. the mechanisms in the structures can be determined by concatenating a unity matrix to right side of $A$ such that a $A \mid I$ new matrix is obtained. Then $A$ is transformed to the echeleon form resulting in a new matrix $\tilde{A} \mid \tilde{I}$. The number of zero-modes or mechanisms in a planar system can be calculated as:

$$m = 2\psi - \kappa - r_A \tag{2}$$

with $r_A$ being the rank of $\tilde{A}$. The number of states of self-stress in a framework can be calculated as:

$$s = \iota - r_A \tag{3}$$

Finally the force components exciting these $m$ zero-modes can be obtained from the left nullspace of $\tilde{A}$ or the bottom $m$ rows of $\tilde{I}$.

## 2.1 Undeformed topology

The undeformed topology can be seen in Figure S2a, left. The equilibrium matrix for the unreformed initial topology can be written as:

$$
A_{\,init} = \begin{pmatrix}
-1 & 0 & 0 & -1 & 0 & 0 & 0 & 0 & 0 & 0 & 0 & 0 & 0 & 0 \\
0 & 0 & 0 & 1.5 & 0 & 0 & 0 & 0 & 0 & 0 & 0 & 0 & 0 & 0 \\
1 & -2 & 0 & 0 & -0.5 & 0 & 0 & 0 & 0 & 0 & 0 & 0 & 0 & 0 \\
0 & 0 & 0 & 0 & 1.5 & 0 & 0 & 0 & 0 & 0 & 0 & 0 & 0 & 0 \\
0 & 2 & -1 & 0 & 0 & 0.5 & 0 & 0 & 0 & 0 & 0 & 0 & 0 & 0 \\
0 & 0 & 0 & 0 & 0 & 1.5 & 0 & 0 & 0 & 0 & 0 & 0 & 0 & 0 \\
0 & 0 & 1 & 0 & 0 & 0 & 1 & 0 & 0 & 0 & 0 & 0 & 0 & 0 \\
0 & 0 & 0 & 0 & 0 & 0 & 1.5 & 0 & 0 & 0 & 0 & 0 & 0 & 0 \\
0 & 0 & 0 & 1 & 0 & 0 & 0 & 1 & 0 & 0 & 0 & 0 & 0 & 0 \\
0 & 0 & 0 & -1.5 & 0 & 0 & 0 & 1.5 & 0 & 0 & 0 & 0 & 0 & 0 \\
0 & 0 & 0 & 0 & 0.5 & 0 & 0 & 0 & 0.5 & 0 & 0 & 0 & 0 & 0 \\
0 & 0 & 0 & 0 & -1.5 & 0 & 0 & 0 & 1.5 & 0 & 0 & 0 & 0 & 0 \\
0 & 0 & 0 & 0 & 0 & -0.5 & 0 & 0 & 0 & -0.5 & 0 & 0 & 0 & 0 \\
0 & 0 & 0 & 0 & 0 & -1.5 & 0 & 0 & 0 & 1.5 & 0 & 0 & 0 & 0 \\
0 & 0 & 0 & 0 & 0 & 0 & -1 & 0 & 0 & 0 & -1 & 0 & 0 & 0 \\
0 & 0 & 0 & 0 & 0 & 0 & -1.5 & 0 & 0 & 0 & 1.5 & 0 & 0 & 0 \\
0 & 0 & 0 & 0 & 0 & 0 & 0 & 0 & -0.5 & 0 & 0 & 1 & -2 & 0 \\
0 & 0 & 0 & 0 & 0 & 0 & 0 & 0 & 0 & 0.5 & 0 & 0 & 2 & -1 \\
0 & 0 & 0 & 0 & 0 & 0 & 0 & 0 & 0 & 0 & 1 & 0 & 0 & 1
\end{pmatrix}
$$

Due to the low connectivity the matrix is sparsely populated. The rank of $A_{init}$ is 14. The structure contains 5 zero-modes (equation 2), and no states of self-stress (equation 3). The force components exciting them are found in the left nullspace ($LNS$) of $\tilde{A}_{\,init}$:

$$
LNS_{\,init} = \begin{pmatrix}
1 & 0 & 0 & 0 & 0 \\
0 & 1 & 0 & 0 & 0 \\
1 & 0 & 0 & 0 & 0 \\
0 & 0 & 1 & 0 & 0 \\
1 & 0 & 0 & 0 & 0 \\
0 & 0 & 0 & 1 & 0 \\
1 & 0 & 0 & 0 & 0 \\
0 & 0 & 0 & 0 & 1 \\
1/2 & -3/4 & 0 & 0 & 0 \\
-1/6 & 1/2 & 0 & 0 & 0 \\
1/2 & 0 & -3/2 & 0 & 0 \\
-1/6 & 0 & 1/2 & 0 & 0 \\
1/2 & 0 & 0 & 3/2 & 0 \\
1/6 & 0 & 0 & 1/2 & 0 \\
1/2 & 0 & 0 & 0 & 3/4 \\
1/6 & 0 & 0 & 0 & 1/2 \\
0 & 0 & 0 & 0 & 0 \\
0 & 0 & 0 & 0 & 0 \\
0 & 0 & 0 & 0 & 0
\end{pmatrix}
$$

Each column in the $LNS$ contains a set of force components acting on the joints which result in inextensional deformation of the structure. For visualization of the zero-modes the coordinates of the joints were displaced by the force component of the $LNS$ as shown in Figure S2b.

## 2.2 Tensile topology

The topology of the structure under tensile deformation is shown in Figure S2a, middle. $A_{tensI}$ is the equilibrium matrix obtained for assuming the self-contact node pairs $E - F$ and $G - H$ are two single nodes. Hence, the number of joints in the structure is reduced by two.

$$A_{tensI} = \begin{pmatrix}
-1 & 0 & 0 & -1.5 & 0 & 0 & 0 & 0 & 0 & 0 & 0 & 0 & 0 & 0 \\
0 & 0 & 0 & 1.5 & 0 & 0 & 0 & 0 & 0 & 0 & 0 & 0 & 0 & 0 \\
1 & -2 & 0 & 0 & -0.5 & 0 & 0 & 0 & 0 & 0 & 0 & 0 & 0 & 0 \\
0 & 0 & 0 & 0 & 1.5 & 0 & 0 & 0 & 0 & 0 & 0 & 0 & 0 & 0 \\
0 & 2 & -1 & 0 & 0 & 0.5 & 0 & 0 & 0 & 0 & 0 & 0 & 0 & 0 \\
0 & 0 & 0 & 0 & 0 & 1.5 & 0 & 0 & 0 & 0 & 0 & 0 & 0 & 0 \\
0 & 0 & 1 & 0 & 0 & 0 & 1.5 & 0 & 0 & 0 & 0 & 0 & 0 & 0 \\
0 & 0 & 0 & 0 & 0 & 0 & 1.5 & 0 & 0 & 0 & 0 & 0 & 0 & 0 \\
0 & 0 & 0 & 1.5 & 0.5 & 0 & 0 & 1.5 & 0.5 & 0 & 0 & 0 & 0 & 0 \\
0 & 0 & 0 & -1.5 & -1.5 & 0 & 0 & 1.5 & 1.5 & 0 & 0 & 0 & 0 & 0 \\
0 & 0 & 0 & 0 & 0 & -0.5 & -1.5 & 0 & 0 & -0.5 & -1.5 & 0 & 0 & 0 \\
0 & 0 & 0 & 0 & 0 & -1.5 & -1.5 & 0 & 0 & 1.5 & 1.5 & 0 & 0 & 0 \\
0 & 0 & 0 & 0 & 0 & 0 & 0 & 0 & -0.5 & 0 & 0 & 1 & -2 & 0 \\
0 & 0 & 0 & 0 & 0 & 0 & 0 & 0 & 0 & 0.5 & 0 & 0 & 2 & -1 \\
0 & 0 & 0 & 0 & 0 & 0 & 0 & 0 & 0 & 0 & 1.5 & 0 & 0 & 1
\end{pmatrix}$$

Alternatively one can model the self-contact pairs in the network as two separate joints with two addition kinematic constrains. The resulting equilibrium matrix $A_{tensII}$ has the same dimensions, but is not identical.

$$A_{tensII} = \begin{pmatrix}
-1 & 0 & 0 & -1.5 & 0 & 0 & 0 & 0 & 0 & 0 & 0 & 0 & 0 & 0 \\
0 & 0 & 0 & 1.5 & 0 & 0 & 0 & 0 & 0 & 0 & 0 & 0 & 0 & 0 \\
1 & -2 & 0 & 0 & -0.5 & 0 & 0 & 0 & 0 & 0 & 0 & 0 & 0 & 0 \\
0 & 0 & 0 & 0 & 1.5 & 0 & 0 & 0 & 0 & 0 & 0 & 0 & 0 & 0 \\
0 & 2 & -1 & 0 & 0 & 0.5 & 0 & 0 & 0 & 0 & 0 & 0 & 0 & 0 \\
0 & 0 & 0 & 0 & 0 & 1.5 & 0 & 0 & 0 & 0 & 0 & 0 & 0 & 0 \\
0 & 0 & 1 & 0 & 0 & 0 & 1.5 & 0 & 0 & 0 & 0 & 0 & 0 & 0 \\
0 & 0 & 0 & 0 & 0 & 0 & 1.5 & 0 & 0 & 0 & 0 & 0 & 0 & 0 \\
0 & 0 & 0 & -1.5 & 0 & 0 & 0 & 1.5 & 0 & 0 & 0 & 0 & 0 & 0 \\
0 & 0 & 0 & 0 & -1.5 & 0 & 0 & 0 & 1.5 & 0 & 0 & 0 & 0 & 0 \\
0 & 0 & 0 & 0 & 0 & -1.5 & 0 & 0 & 0 & 1.5 & 0 & 0 & 0 & 0 \\
0 & 0 & 0 & 0 & 0 & 0 & -1.5 & 0 & 0 & 0 & 1.5 & 0 & 0 & 0 \\
0 & 0 & 0 & 0 & 0 & 0 & 0 & 0 & -0.5 & 0 & 0 & 1 & -2 & 0 \\
0 & 0 & 0 & 0 & 0 & 0 & 0 & 0 & 0 & 0.5 & 0 & 0 & 2 & -1 \\
0 & 0 & 0 & 0 & 0 & 0 & 0 & 0 & 0 & 0 & 1.5 & 0 & 0 & 1
\end{pmatrix}$$

Both matrices have the rank 14 and the same left nullspace. From this it can be concluded that the network behaves identical for both approaches of describing the self-contact joints.

$$
LNS_{\ tens} = \begin{pmatrix} 1 \\ 1 \\ 1 \\ 1/3 \\ 1 \\ -1/3 \\ 1 \\ -1 \\ 0 \\ 0 \\ 0 \\ 0 \\ 0 \\ 0 \\ 0 \end{pmatrix}
$$

Since the rank is 14, the structure contains one zero-mode, which is excited by the force components of the $LNS_{\ tens}$, and again no states of self-stress. The joint coordinates displaced by the components is shown in Figure S2c.

## 2.3 Compression topology

The topology arising from compressive deformation is shown in Figure S2a, right. One self-contact node has formed, which can again be described as one single node $F = G$ ($I$), or as additional constrains of nodes $F$ and $G$ in the x-direction ($II$). The equilibrium matrices for the two cases are the following:

$$
A_{\ compI} = \begin{pmatrix}
-1 & 0 & 0 & -1 & 0 & 0 & 0 & 0 & 0 & 0 & 0 & 0 & 0 & 0 \\
0 & 0 & 0 & 1.5 & 0 & 0 & 0 & 0 & 0 & 0 & 0 & 0 & 0 & 0 \\
1 & -2 & 0 & 0 & -1 & 0 & 0 & 0 & 0 & 0 & 0 & 0 & 0 & 0 \\
0 & 0 & 0 & 0 & 1.5 & 0 & 0 & 0 & 0 & 0 & 0 & 0 & 0 & 0 \\
0 & 2 & -1 & 0 & 0 & 1 & 0 & 0 & 0 & 0 & 0 & 0 & 0 & 0 \\
0 & 0 & 0 & 0 & 0 & 1.5 & 0 & 0 & 0 & 0 & 0 & 0 & 0 & 0 \\
0 & 0 & 1 & 0 & 0 & 0 & 1 & 0 & 0 & 0 & 0 & 0 & 0 & 0 \\
0 & 0 & 0 & 0 & 0 & 0 & 1.5 & 0 & 0 & 0 & 0 & 0 & 0 & 0 \\
0 & 0 & 0 & 1 & 0 & 0 & 0 & 1 & 0 & 0 & 0 & 0 & 0 & 0 \\
0 & 0 & 0 & -1.5 & 0 & 0 & 0 & 1.5 & 0 & 0 & 0 & 0 & 0 & 0 \\
0 & 0 & 0 & 0 & 1 & -1 & 0 & 0 & 1 & -1 & 0 & 0 & 0 & 0 \\
0 & 0 & 0 & 0 & -1.5 & -1.5 & 0 & 0 & 1.5 & 1.5 & 0 & 0 & 0 & 0 \\
0 & 0 & 0 & 0 & 0 & 0 & -1 & 0 & 0 & 0 & -1 & 0 & 0 & 0 \\
0 & 0 & 0 & 0 & 0 & 0 & -1.5 & 0 & 0 & 0 & 1.5 & 0 & 0 & 0 \\
0 & 0 & 0 & 0 & 0 & 0 & 0 & 0 & -1 & 0 & 0 & 1 & -2 & 0 \\
0 & 0 & 0 & 0 & 0 & 0 & 0 & 0 & 0 & 1 & 0 & 0 & 2 & -1 \\
0 & 0 & 0 & 0 & 0 & 0 & 0 & 0 & 0 & 0 & 1 & 0 & 0 & 1
\end{pmatrix}
$$

$$
A_{compII} = \begin{pmatrix}
-1 & 0 & 0 & -1 & 0 & 0 & 0 & 0 & 0 & 0 & 0 & 0 & 0 & 0 \\
0 & 0 & 0 & 1.5 & 0 & 0 & 0 & 0 & 0 & 0 & 0 & 0 & 0 & 0 \\
1 & -2 & 0 & 0 & -1 & 0 & 0 & 0 & 0 & 0 & 0 & 0 & 0 & 0 \\
0 & 0 & 0 & 0 & 1.5 & 0 & 0 & 0 & 0 & 0 & 0 & 0 & 0 & 0 \\
0 & 2 & -1 & 0 & 0 & 1 & 0 & 0 & 0 & 0 & 0 & 0 & 0 & 0 \\
0 & 0 & 0 & 0 & 0 & 1.5 & 0 & 0 & 0 & 0 & 0 & 0 & 0 & 0 \\
0 & 0 & 1 & 0 & 0 & 0 & 1 & 0 & 0 & 0 & 0 & 0 & 0 & 0 \\
0 & 0 & 0 & 0 & 0 & 0 & 1.5 & 0 & 0 & 0 & 0 & 0 & 0 & 0 \\
0 & 0 & 0 & 1 & 0 & 0 & 0 & 1 & 0 & 0 & 0 & 0 & 0 & 0 \\
0 & 0 & 0 & -1.5 & 0 & 0 & 0 & 1.5 & 0 & 0 & 0 & 0 & 0 & 0 \\
0 & 0 & 0 & 0 & -1.5 & 0 & 0 & 0 & 1.5 & 0 & 0 & 0 & 0 & 0 \\
0 & 0 & 0 & 0 & 0 & -1.5 & 0 & 0 & 0 & 1.5 & 0 & 0 & 0 & 0 \\
0 & 0 & 0 & 0 & 0 & 0 & -1 & 0 & 0 & 0 & -1 & 0 & 0 & 0 \\
0 & 0 & 0 & 0 & 0 & 0 & -1.5 & 0 & 0 & 0 & 1.5 & 0 & 0 & 0 \\
0 & 0 & 0 & 0 & 0 & 0 & 0 & 0 & -1 & 0 & 0 & 1 & -2 & 0 \\
0 & 0 & 0 & 0 & 0 & 0 & 0 & 0 & 0 & 1 & 0 & 0 & 2 & -1 \\
0 & 0 & 0 & 0 & 0 & 0 & 0 & 0 & 0 & 0 & 1 & 0 & 0 & 1
\end{pmatrix}
$$

As for the tensile topology the two equilibrium matrices have the same rank ($r_A = 14$), resulting in $m = 3$ mechanisms and $s = 0$ states of self stress. Again the left nullspace of both matrices contains the same force components:

$$
LNS_{comp} = \begin{pmatrix}
1 & 0 & 0 \\
0 & 1 & 0 \\
1 & 0 & 0 \\
2/3 & 0 & 0 \\
1 & 0 & 0 \\
-2/3 & 0 & 0 \\
1 & 0 & 0 \\
0 & 0 & 1 \\
1/2 & -3/4 & 0 \\
-1/3 & 1/2 & 0 \\
0 & 0 & 0 \\
0 & 0 & 0 \\
1/2 & 0 & 3/4 \\
1/3 & 0 & 1/2 \\
0 & 0 & 0 \\
0 & 0 & 0 \\
0 & 0 & 0
\end{pmatrix}
$$

The visualization of these force components is shown in Figure S2d.

# 3 Numerical simulations of the topological transitions

Numerical simulations of the metamaterials are performed to investigate the transition in topology and its influence on the mechanical response. The graphs of Figure S3 show the simulated bodies corresponding to the stress-strain curves shown in Figure 3 of the original article. It is clearly visible that stresses are transmitted across the contacts formed.

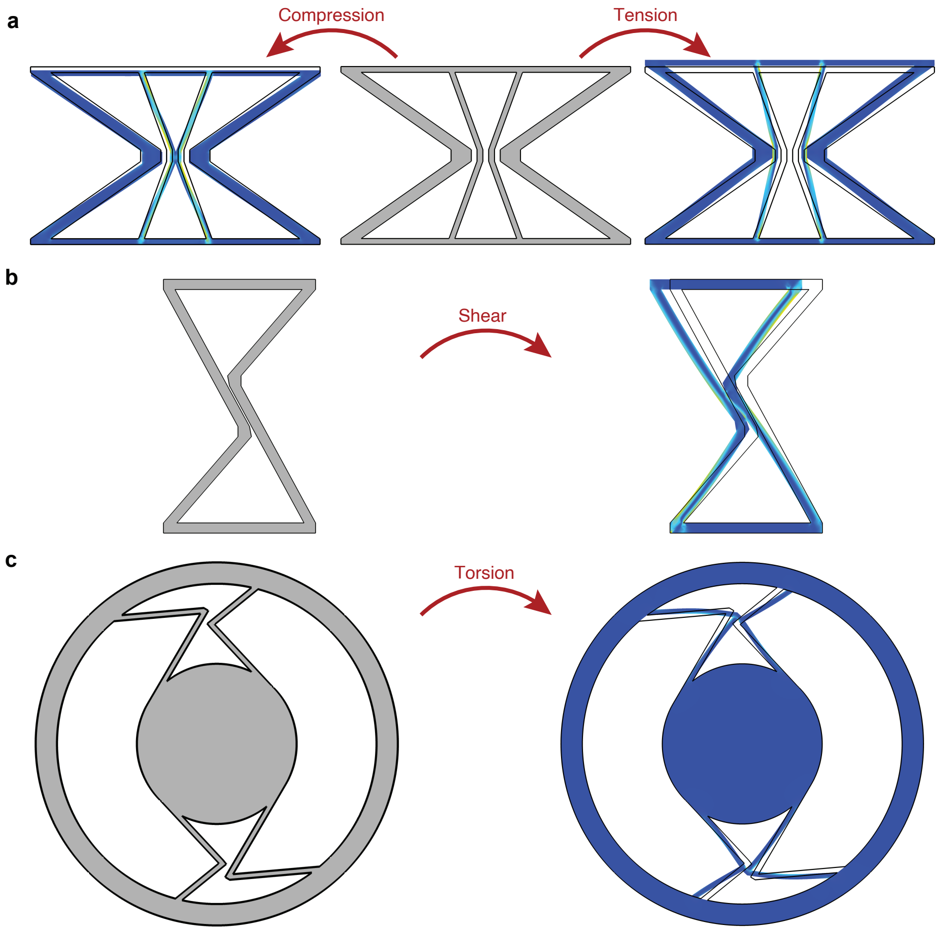


Figure S3: Topological states of the tension and compression (a), shear (b), and torsion (c) metamaterial obtained from numerical simulations. The color code indicates the von Mises stress.

# 4 Modification of the unit cell

The unit cell of the tension / compression metamaterial is modified to increase the number of contacts when deformed. This leads to an increase in the $r$ ratio between the moduli. Figure S4 shows the simulated stress strain curves of two metamaterials consisting of 3 by 3 unit cells, comparing the simple unit cell to the modified one. Both unit cells have identical design parameters.

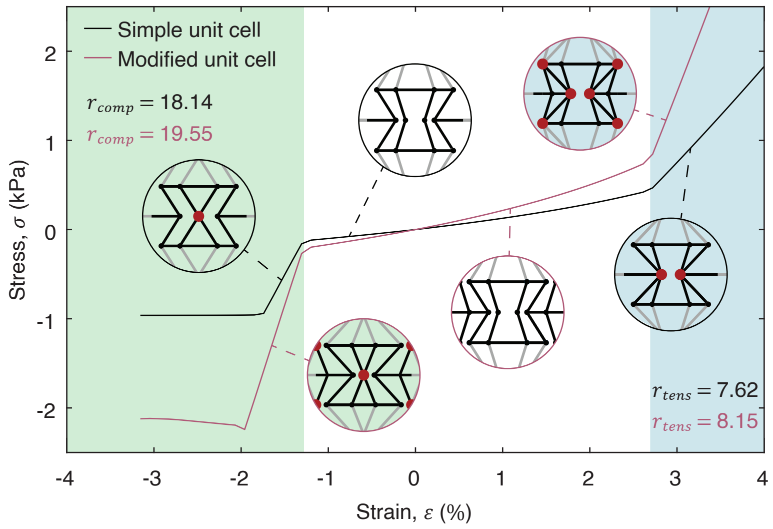


Figure S4: Simulated mechanical response of a metamaterial of the simple (black) and modified (magenta) unit cell. The increased number of contacts results an a larger elastic nonlinearity.

## 5 One-dimensional Betti number as a metric to describe transitions in nodal-topology

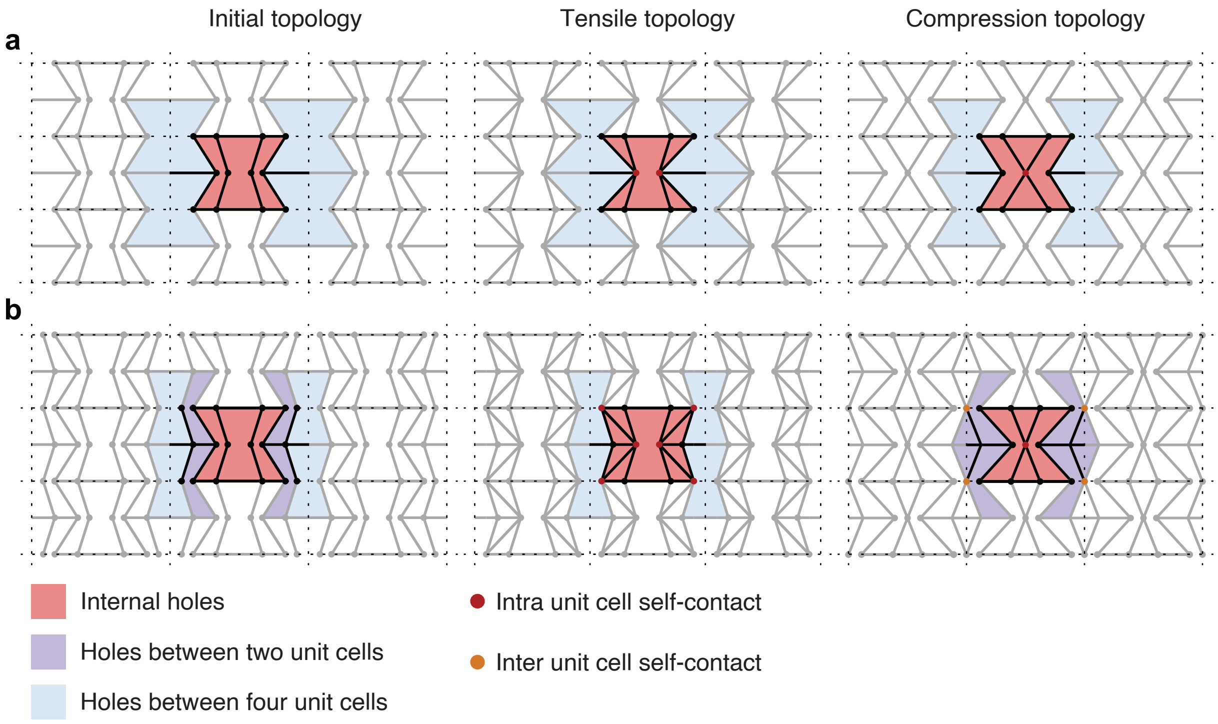


Figure S5: Illustration of holes formed by one unit cell in a periodic lattice. The number of self contacts and hence the magnitude of the topology transition can be increased by adapting the unit cell from (a) as it is shown in (b). The one- dimensional Betti number per unit cell is determined by counting the closed holes formed by the beams of a unit cell. Holes formed between two neighboring unit cell are counted as halve and holes formed by beams of four different unit cells are counted as one fourth.

Here, we suggest employing the Betti numbers to describe the different topological states. The

Betti numbers describe the topologies of n-dimensional simplicial complexes. When applied to the planar representations of our metamaterials, the change in the topology can be described by the one-dimensional Betti number $b_1$, which is the number of holes in a topology. The change in the Betti number between the different states can serve as a measure for the change in nodal-topology. To exemplify this, we shall have a look at the unit cells of our metamaterials. For the tensile / compression metamaterial in the undeformed state (original article Figure 1a), we find $b_1$ = 3, as the beams form three holes which are separate from one another. Under tensile deformation the Betti number increases to $b_1$ = 5 and in compression to $b_1$ = 4. Hence, we find $\Delta b_{1t} = 2$ and $\Delta b_{1c} = 1$. The same observations can be made for the shear metamaterial (original article Figure 1b), where $b_1$ increases from 1 to 2, and the torsion metamaterial (original article Figure 1c) increasing from 4 to 6.
In a periodic assembly the Betti number per unit cell changes due to holes formed with neighboring unit cells. Holes formed between two unit cells are counted halve and the number of holes formed between four unit cells is divided by four. The unit cell as it is shown in Figure 1a (original article) in a periodic assembly possess the same Betti numbers as discussed before, plus 1 in each state to account for the $4/4 = 1$ holes formed with the neighboring unit cells (see Figure S5a). The change in topology is again $\Delta b_{1c} = 1$ in the compression state and $\Delta b_{1t} = 2$ in the tension state. To maximize the change in topology, i.e. $\Delta b_1$, the unit cell was adapted as shown in Figure S7. The number of intra unit cell self-contact nodes formed in tension increases from 2 to 6. In compression there is an increase from 1 intra unit cell, to 1 intra unit cell and 4 inter unit cell self-contact nodes. As a result, the Betti number increases to 6 in the initial state, 8 in the compression state, and 10 in the tension state. For the adapted unit cell (Figure S1b), the relative change in the Betti number between the different topological states is doubled compared with the simple unit cell (Figure S1a) ($\Delta b_{1c} = 2$, $\Delta b_{1t} = 4$). The Betti number can be used as a criterion to design topological changing metamaterials. An increase in the one-dimensional Betti number ($\Delta b_1 > 0$) is a necessary condition for a change from a soft to a rigid mode of deformation in mechanical metamaterials. However a sufficient condition is not provided. This requires computing the soft modes by linear algebraic analysis as shown in section 2.

# 6 Metamaterial unit cells in periodic assembly

Metamaterials can be created from the unit cells introduced in the original article Figure 1 by tessellating as shown in Figure S6. Note that while the tension / compression and torsion metamaterial can be tessellated simply in x- and y-direction, the shear metamaterial requires a more complex shifting between neighboring unit cells. The tension / compression metamaterial (left) is made from the modified unit cell as discussed in section 5 and shown in section 7.

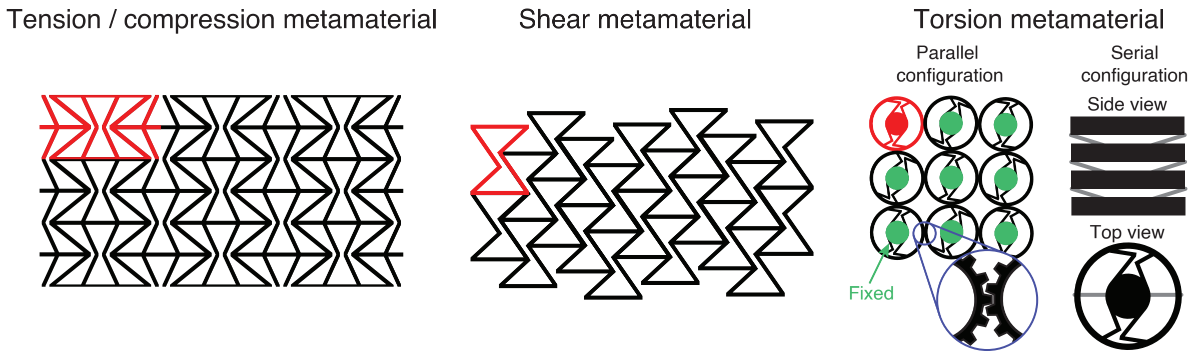


Figure S6: Tessellations of unit cells of the tension/compression, shear, and torsion metamaterial. The unit cells are highlighted in red.

# 7 Parametric design

## 7.1 Tension / compression metamaterial

The design parameters necessary to define the unit cell of the tension / compression type mechanical metamaterial is shown in Figure S7. Independent parameters which can be chosen to alter the unit cell are shown in black. Dependent design parameters are shown in red and can be calculated according to equation 4 - 8.

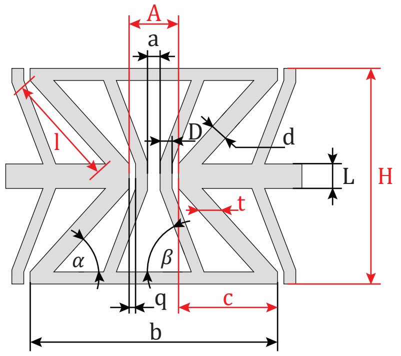


Figure S7: Unit cell of the tension/compression metamaterial. The independent design parameters are shown in black, dependent design parameters are shown in red.

$$A = a + 2\,D + 2\,q \tag{4}$$

$$t = \frac{d}{sin(\alpha)} \tag{5}$$

$$l = \frac{b - A - 2\,t}{2\,cos(\alpha)} \tag{6}$$

$$H = 2\,sin(\alpha) * l + 2\,L \tag{7}$$

$$c = \frac{b - A}{2} \tag{8}$$

## 7.2 Design parameters of numerical simulations and experimental testing

The design parameters used in the numerical simulations are shown in the tables in this section. Parameters which are swept are written as lower bound , step size , upper bound.

Table 1: Parameters for the $\alpha$ - $\beta$ sweep, with the condition that $\beta \geq \alpha$.

| $\alpha$ [°] | $\beta$ [°] | $L$ [$mm$] | $a$ [$mm$] | $D$ [$mm$] | $d$ [$mm$] | $q$ [$mm$] | $b$ [$mm$] |
|---|---|---|---|---|---|---|---|
| [30,5,70] | [50,5,80] | 2.0 | 1.0 | 1.0 | 2.0 | 1.0 | 50 |

Table 2: Parameters for the $a$ - $\beta$ sweep.

| $\alpha$ [°] | $\beta$ [°] | $L$ [$mm$] | $a$ [$mm$] | $D$ [$mm$] | $d$ [$mm$] | $q$ [$mm$] | $b$ [$mm$] |
|---|---|---|---|---|---|---|---|
| 35 | [50,5,80] | 2.0 | [0.5,0.1,1.5] | 1.0 | 2.0 | 1.0 | 50 |

Table 3: Parameters for the $\alpha$ - $q$ sweep.

| $\alpha$ [°] | $\beta$ [°] | $L$ [$mm$] | $a$ [$mm$] | $D$ [$mm$] | $d$ [$mm$] | $q$ [$mm$] | $b$ [$mm$] |
|---|---|---|---|---|---|---|---|
| [30,5,70] | 70 | 2.0 | 1.0 | 1.0 | 2.0 | [0.5,0.1,1.5] | 50 |

Table 4: Parameters for the $D$ / $d$ sweep.

| $\alpha$ [°] | $\beta$ [°] | $L$ [$mm$] | $a$ [$mm$] | $D$ [$mm$] | $d$ [$mm$] | $q$ [$mm$] | $b$ [$mm$] |
|---|---|---|---|---|---|---|---|
| 35 | 70 | 2.0 | 1.0 | [0.5,0.1,3.0] | 2×$D$ | 1.0 | 50 |

Table 5: Parameters of the 3D printed and experimentally tested specimen.

| $\alpha$ [°] | $\beta$ [°] | $L$ [$mm$] | $a$ [$mm$] | $D$ [$mm$] | $d$ [$mm$] | $q$ [$mm$] | $b$ [$mm$] |
|---|---|---|---|---|---|---|---|
| 35 | 70 | 1.0 | 2.0 | 1.0 | 2.0 | 1.0 | 50 |

# 8 Meta-structures with programmable deformation

By combining unit cells with different contact strains and different stiffness after contact, one can design meta-structures with designed deformation. Figure S8 shows an example of such a structure. A 2×5 system of unit cells has been assembled according to the schematic in Figure S8 a. Under compression, topological transitions first occur in locally confined region (blue), leading to lateral deflection. Note that in the final compressed state all unit cells have changed the topology. In this design, the simple unit cell is used. The modified unit cell from section 5 would not form inter-unit cell contacts due to the bending component of the unit cell deformation.

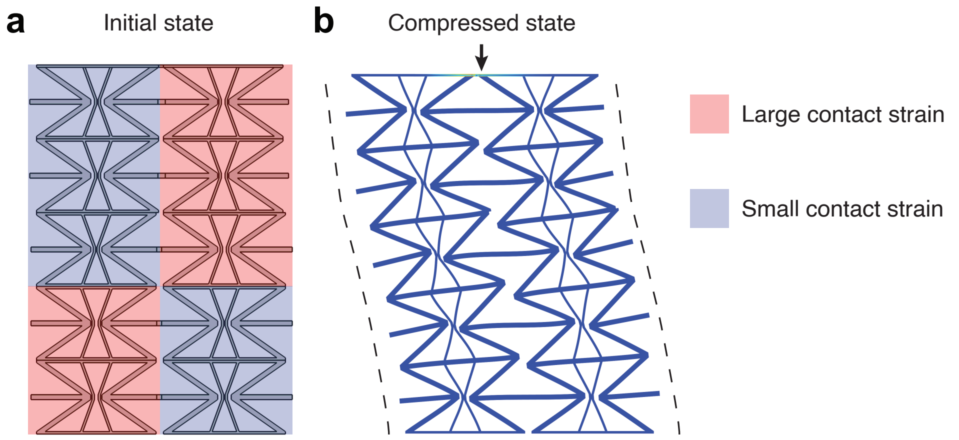


Figure S8: Tower of 5×2 unit cells. a) Initial configuration with assembled unit cells of high and low contact strain. b) In the deformed configuration the tower leans to the left as the topological transition of the two bottom left unit cells takes place at larger strains.

# References

[1] Sergio Pellegrino and Christopher Reuben Calladine. "Matrix analysis of statically and kinematically indeterminate frameworks". In: *International Journal of Solids and Structures* 22.4 (1986), pp. 409–428. ISSN: 0020-7683.
